# Supplementary material for: Rapid Computation of Thermodynamic Properties Over Multidimensional Nonbonded Parameter Spaces using Adaptive Multistate Reweighting
Source: arXiv:1509.02560 source file (2015-09-08)
Supplement: Supplementary file 1 [file NadenShirtsBasis3Sup.pdf]

# Supplementary Material for "Rapid Computation of Thermodynamic Properties Over Multidimensional Nonbonded Parameter Spaces using Adaptive Multistate Reweighting"

Levi N. Naden and Michael R. Shirts*

*Department of Chemical Engineering, University of Virginia, Charlottesville, Virginia 22904, USA*

E-mail: michael.shirts@virginia.edu

*To whom correspondence should be addressed

## S.1 Considerations for solvents with multiple unique particles

One complication to the linear basis representation approach is when the solvent is composed of multiple particle types. Situations where this happens includes both solvents with multiple types of molecules, and solvents where multiple atom types make up each solvent molecule, such as water. A different set of scalar alchemical switches, $h_n(\lambda_n)$, for each unique atom type in the solvent is required to accurately compute the energies for arbitrary state $Z$. This is because we are only changing $\sigma_{ii}$ of the solute explicitly, but $C_{12}$ and $C_6$ will scale as non-linear functions of $\sigma_{ij}$, which will be different for the interactions with each solvent atom type. One solution is to compute the basis functions for each solvent atom type interacting with the solute. However, this can be avoided with geometric mixing rules for both Lennard-Jones parameters,

$$\varepsilon_{ij} = \left(\varepsilon_{ii}\varepsilon_{jj}\right)^{1/2}$$
$$\sigma_{ij} = \left(\sigma_{ii}\sigma_{jj}\right)^{1/2}$$

as opposed to arithmetic mixing rules for $\sigma_{ij}$, where $\sigma_{ij} = 0.5(\sigma_{ii} + \sigma_{jj})$. It is important to note that Eq. 6 is still valid for arithmetic mixing rules, but requires a separate $C_{12}$ and $C_6$ term for each atom type in the solvent. Alternatively, the arithmetic mixing rules could undergo binomial expansion as

$$\left[\frac{1}{2}(\sigma_{ii} + \sigma_{jj})\right]^n = \frac{1}{2^n}\sum_{\ell=0}^{n}\binom{n}{\ell}\sigma_{ii}^{n-\ell}\sigma_{ij}^{\ell} \tag{S.1}$$

and new $h_n(\lambda_n)$ functions written which scale each $\sigma_{ii}^{n-\ell}$ term. The potential of any atom can be computed with geometric mixing rules and two reference points. This section will denote each $C_n$ explicitly in terms of the reference particles, $X$ and $Y$, and the arbitrary solvent site $S$, where $S$ can represent any of the solvent particles as they will cancel out of the equations.

We can represent Coulombic and geometric Lennard-Jones mixing rules of the $C_n$ terms by a general form of

$$C_{n,ij} = \left(C_{n,ii}C_{n,jj}\right)^m \tag{S.2}$$

where $m$ takes discrete values of $1/2$ or or 1 depending on the index of $\ell$. For our basis functions, the $C_{12}$ and $C_6$ terms have $m = 1/2$, whereas the electrostatic basis is $m = 1$ since its mixing term is $q_i q_j$. Representing the mixing rules in this way is beneficial as the following derivation does not depend on the exact value of $m$. Eq. 6 can be expanded as

$$u(r,\lambda) = u_{\text{unaffected}} + \sum_{\ell} \left[ \frac{h_n(\lambda_n)\left(C_{n,YS} - C_{n,XS}\right) + C_{n,XS}}{r^n} \right]_{\ell}$$
$$u(r,\lambda) = u_{\text{unaffected}} + \sum_{\ell} \left[ \frac{h_n(\lambda_n)\left[\left(C_{n,YY}C_{n,SS}\right)^m - \left(C_{n,XX}C_{n,SS}\right)^m\right] + \left(C_{n,XX}C_{n,SS}\right)^m}{r^n} \right]_{\ell} . \quad \text{(S.3)}$$

We know that for any arbitrary state $Z$ that

$$\left(C_{n,ZZ}C_{n,SS}\right)^m = h_n(\lambda_n)\left[\left(C_{n,YY}C_{n,SS}\right)^m - \left(C_{n,XX}C_{n,SS}\right)^m\right] + \left(C_{n,XX}C_{n,SS}\right)^m . \quad \text{(S.4)}$$

We can determine what value $h_n(\lambda_n)$ should take given a $C_{n,ZZ}$ from Eq. (S.4) by

$$h_n = \frac{C^m_{n,ZZ} - C^m_{n,XX}}{C^m_{n,YY} - C^m_{n,XX}} . \quad \text{(S.5)}$$

Because we are using multiplicative mixing rules, Eq. (S.5) does not depend on any solvent parameter or site. The potential of any configuration evaluated at state $Z$ can then be computed from the basis functions[1] and Eq. 6.

## S.2 Relative free energies for uncharged, chemically realistic Lennard-Jones spheres

Solvation simulations for chemically realistic Lennard-Jones (LJ) spheres were carried out to validate the parameter search approach. The LJ spheres tested were united atom (UA) methane,[2–4] neopentane,[5] and an approximation for a $C_{60}$ molecule.[1] This simulations were carried out under the same conditions as in Section 3 with the addition of sampling along a fixed thermodynamic

path. Solvation simulations were carried out per sphere along the a soft core coupling path[6,7] with a 1-1-6 parameterization.[1,8,9] $\lambda$ was along this path was sampled at 11 uniformly placed states from $\lambda = 0$ to $\lambda = 1$.

Table S.1: Relative free energies are statistically indistinguishable between solvation simulations and those computed from the basis function search of nonbonded parameter space. The free energy of solvation each particle was simulated (Direct Solvation) and the relative free energy to the reference state was computed (Relative Solvation). The Relative Solvation was compared to the relative free energy computed from the parameter search with 12 states of collected data (Parameter Search). The values for Relative Solvation are consistent with the statistical uncertainty for the Parameter Search free energy for the tested particles. Free energy is in units of kcal/mol.

| Molecule | Direct Solvation | Relative Solvation | Parameter Search |
|---|---|---|---|
| Reference Particle | 10.331 ± 0.128 | 0.000 ± 0.000 | 0.000 ± 0.000 |
| UA Methane | 2.215 ± 0.149 | -8.116 ± 0.197 | -7.696 ± 0.083 |
| Neopentane | -0.264 ± 0.093 | -10.595 ± 0.159 | -10.758 ± 0.019 |
| $C_{60}$ | 8.175 ± 0.135 | -2.157 ± 0.186 | -2.318 ± 0.004 |

## S.3 Adaptive sampling algorithm for 3-D parameter search

Identifying multiple regions of phase space which are locally connected, but not globally connected is done by clustering grid points in the multidimensional space based on the relative uncertainty. The algorithm is available on GitHub[10] and details for the algorithm is as follows:

1. Compute the free energy ($\Delta F$) and uncertainty ($\delta\Delta F$) at every grid point in the multidimensional space with MBAR.[11]

2. Choose the subset of grid points, $S$, where $\delta\Delta F$is larger than a threshold uncertainty. We chose the grid points in $S$ such that $\delta\Delta F \geq 0.5\,\mathrm{kcal/mol} \in S$.

3. The DBSCAN[12] clustering algorithm is run on each grid point in $S$ with the following neighbor and neighborhood criteria

   - Neighbor grid point is adjacent to current point, including diagonals

- Relative error in the uncertainty of current point and the neighbor point is $< 10\%$. This must also be true for the relative error in uncertainty of the neighbor point with the current point.
- A minimum of 5 points is required to defined a neighborhood, $N$.

4. Define the number of grid points in each $N_i$ neighborhood as $C_i$

5. Select the "large" neighborhoods, $L$, where "large" is defined by $C_i/\sum_i C_i > 10\%$. This is done to minimize sampling small clusters which may be eliminated on subsequent iterations due to improved phase space overlap from sampling the large clusters.

   In the event no large clusters are identified, the three largest neighborhoods are selected instead.

   In the event that **zero** clusters are identified, reduce the error threshold until 1/3 of the total points are above the threshold. This should allow new clusters to be found while also continuing to lower the uncertainty. Repeat the clustering step.

6. Identify the boundaries in each dimension for each $L_j$ cluster. We choose to use SciPy's[13] multidimensional image analysis module, ndimage. A separate index, $j$, loops over $L$ to account for the fact that $L \subseteq N$.

7. Select a point inside each $L_j$ to perform additional sampling.

   One option is the center of "mass", where the "mass" is the uncertainty of each grid point in $L_j$.

   Alternately, a random point can be selected as was done for this study. Choosing only the center of mass was observed to improve local phase space overlap, but be slow at improving global phase space overlap since the center of mass is often far away from the boundary of $L_j$.

8. Let each point found in the previous step be a vertex, $v_j$ in a graph. Let the reference state

that relative thermodynamic properties are measured with respect to also be a vertex, $R$. Define the superset of all vertices, $V$, such that $V = \{v, R\}$.

9. Create a complete graph of $V$.

10. Find the minimum spanning tree (MST) of the complete graph of $V$. This was done with Kruskal's algorithm[14] here. Distance is defined by the Euclidean distance in multidimensional space.

    The MST creates a network of edges along where we will expand the local phase space overlap from each $L$, while also minimizing total number of edges required. So long as there is any path of phase space overlap connecting two states; converged, low uncertainty estimates of thermodynamic properties can be made.

11. Compute the error along regularly spaced points on each edge of the MST with multidimensional interpolation from nearby grid points. The points along the edge do not have to reside along the regular spaced grid.

12. Run a boundary detection algorithm on each edge in the MST to identify the boundary of the local phase space overlap. We chose the the Sobel boundary detection algorithm.[15]

13. The new states to sample are then each point of the vertices, $v$, and each boundary found along the edges of the MST.

## S.4 Ion Radial Distribution Functions

This section has the estimated radial distribution functions (RDFs, $g(r)$) for each ion from the Joung and Cheatham set in TIP3P water.[16] The RDFs are estimated at 160 evenly spaced bins from $r = 0$ to $r = 12$ nm from 203 sampled states of data. We have provided the Python code used to compute the RDFs on GitHub.[10] The following RDFs are the Ion-Water Oxygen pair distances estimated by MBAR[11] with error shown as dashed lines around the curve black lines. The green

lines are the RDFs computed by directly simulating the ion and estimating the RDF from the trajectory. Error in the green lines is shown as dashed lines around the curve and estimated from 200 bootstrap samples of the simulated data.[17] The data from these direct simulations were not used in the MBAR estimate. The $Li^{+}$ and $Na^{+}$ $\sigma_{ii}$ are are below the searched parameter space, leading to their RDFs appearing erratic and falling below $g(r) = 0$.

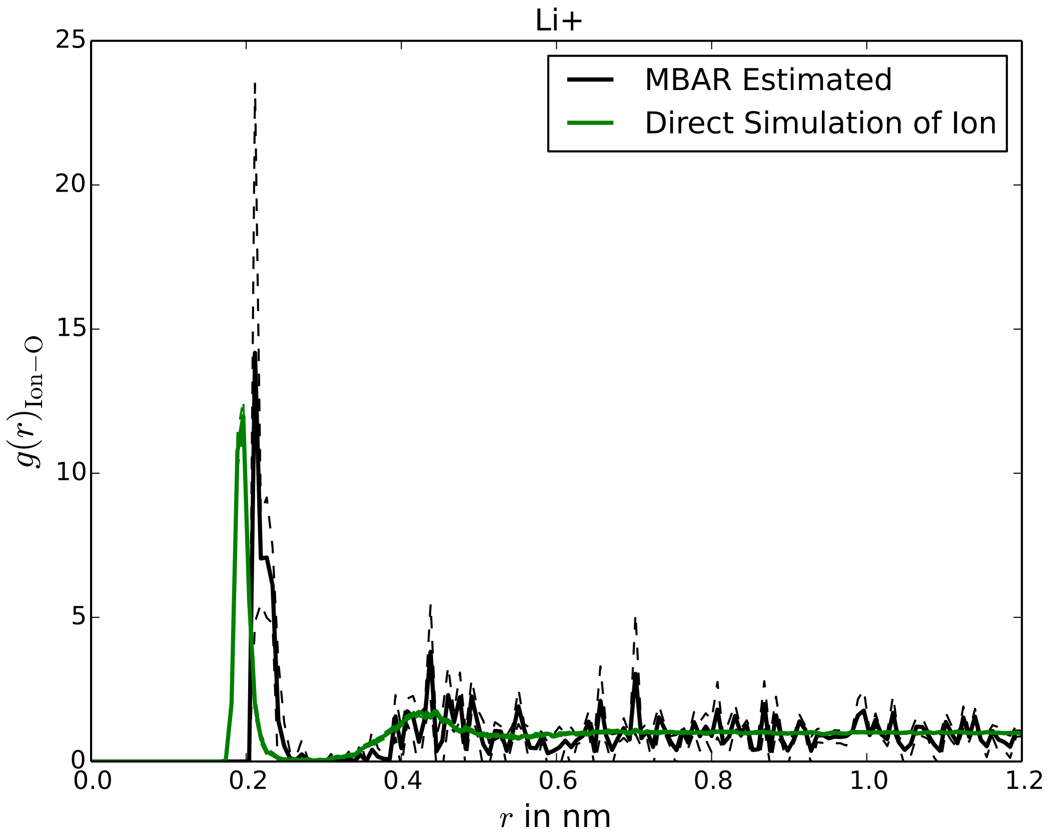


Figure S.1: RDF for $Li^{+}$, this is also Fig. 8b

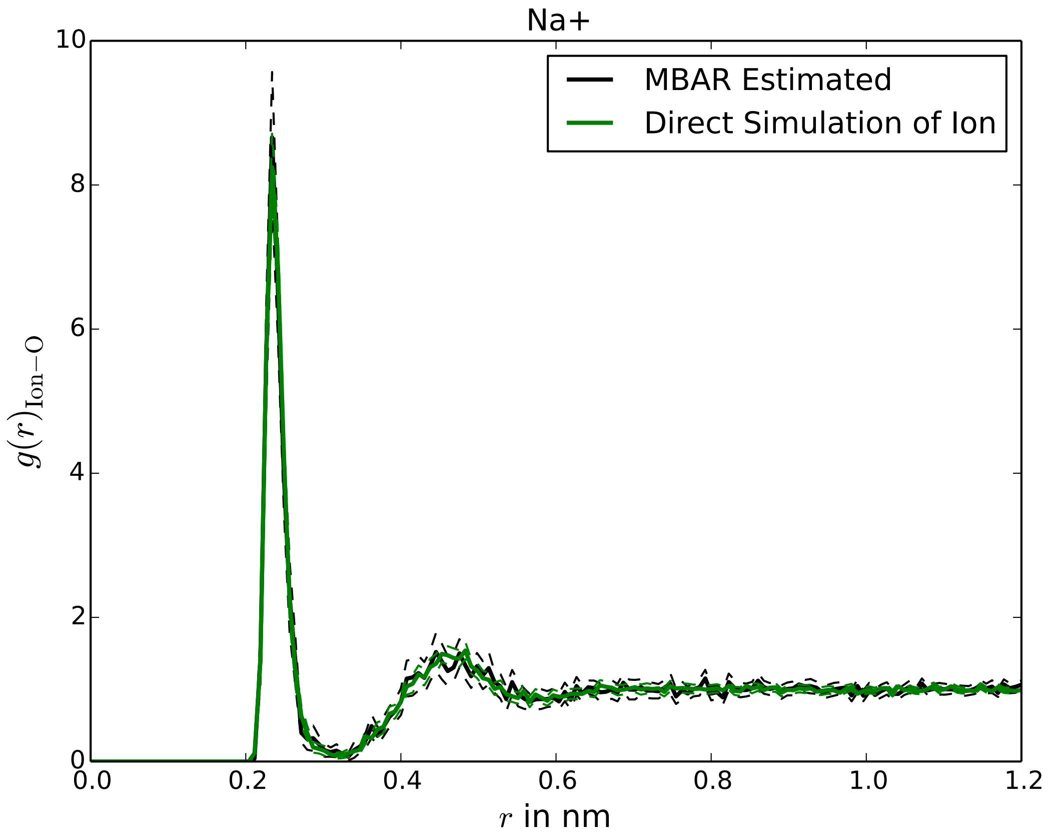


Figure S.2: RDF for $Na^+$

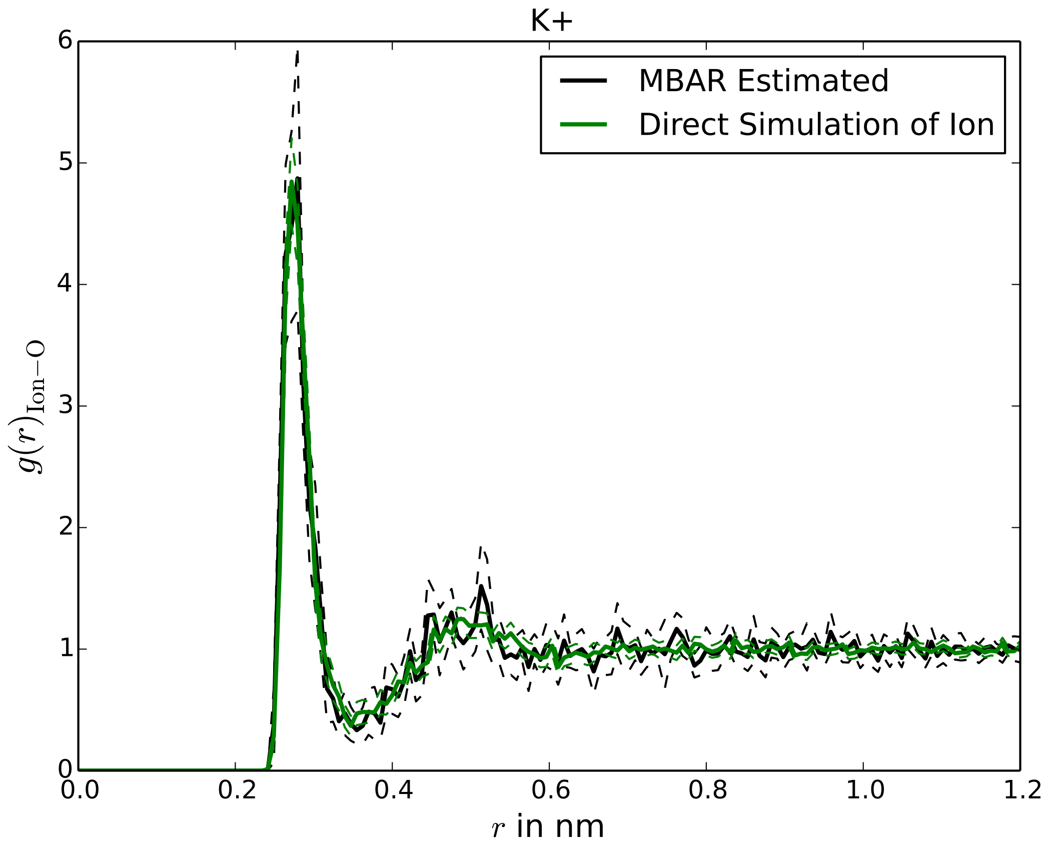


Figure S.3: RDF for $K^+$

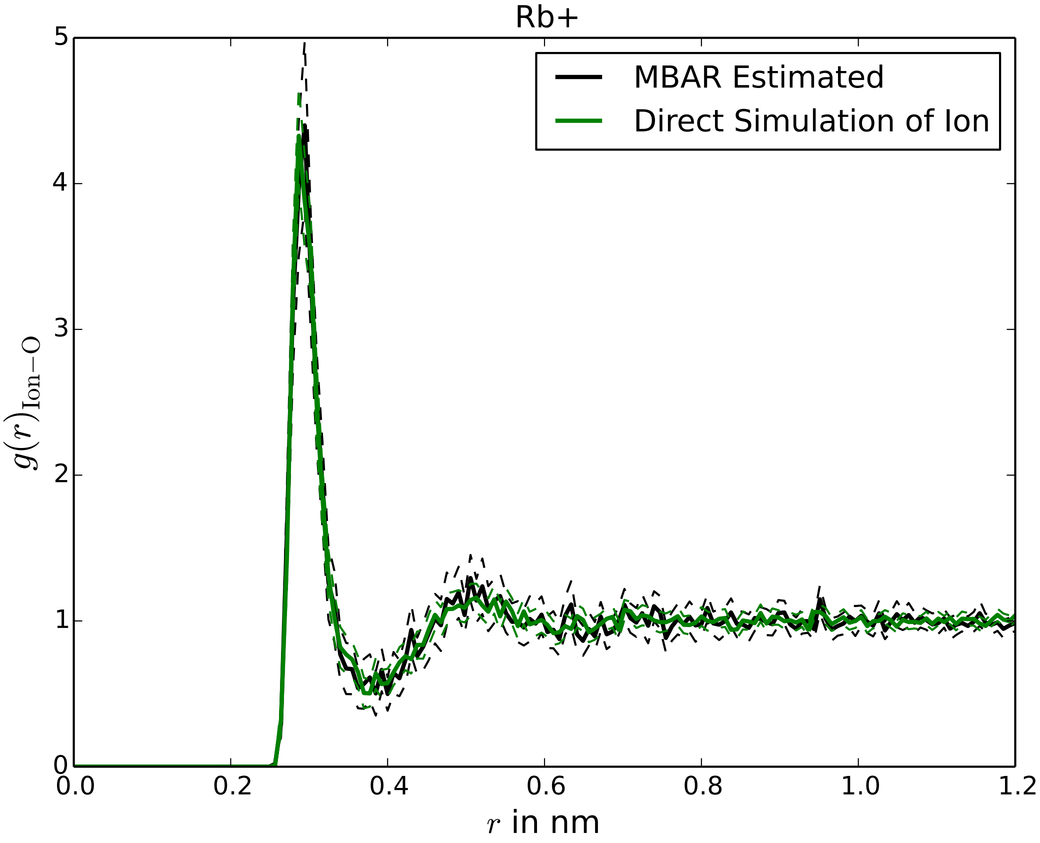


Figure S.4: RDF for $Rb^{+}$

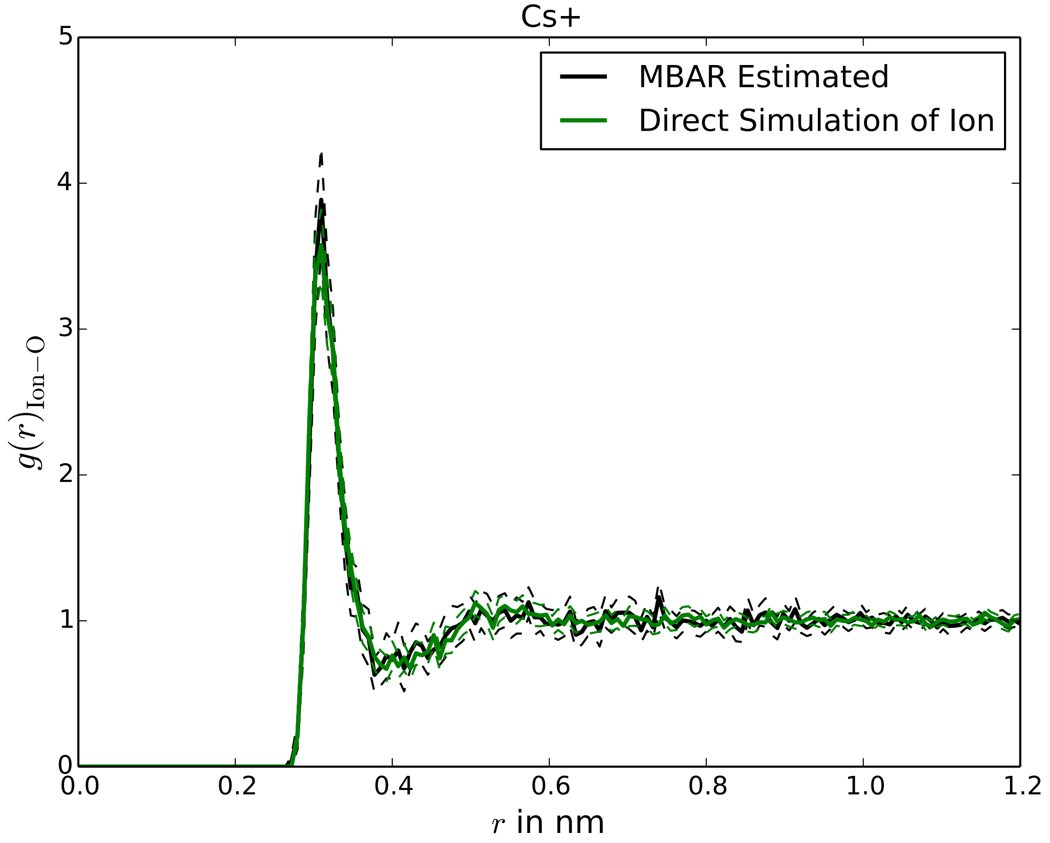


Figure S.5: RDF for $Cs^{+}$

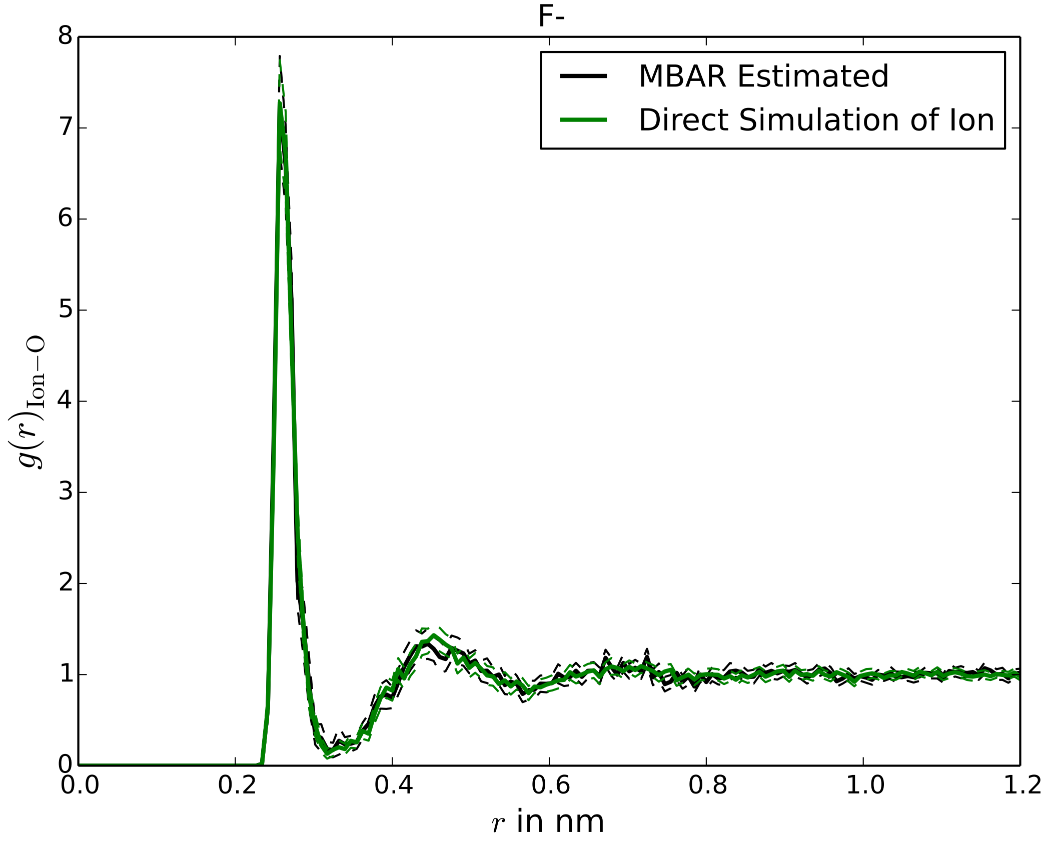


Figure S.6: RDF for $F^-$

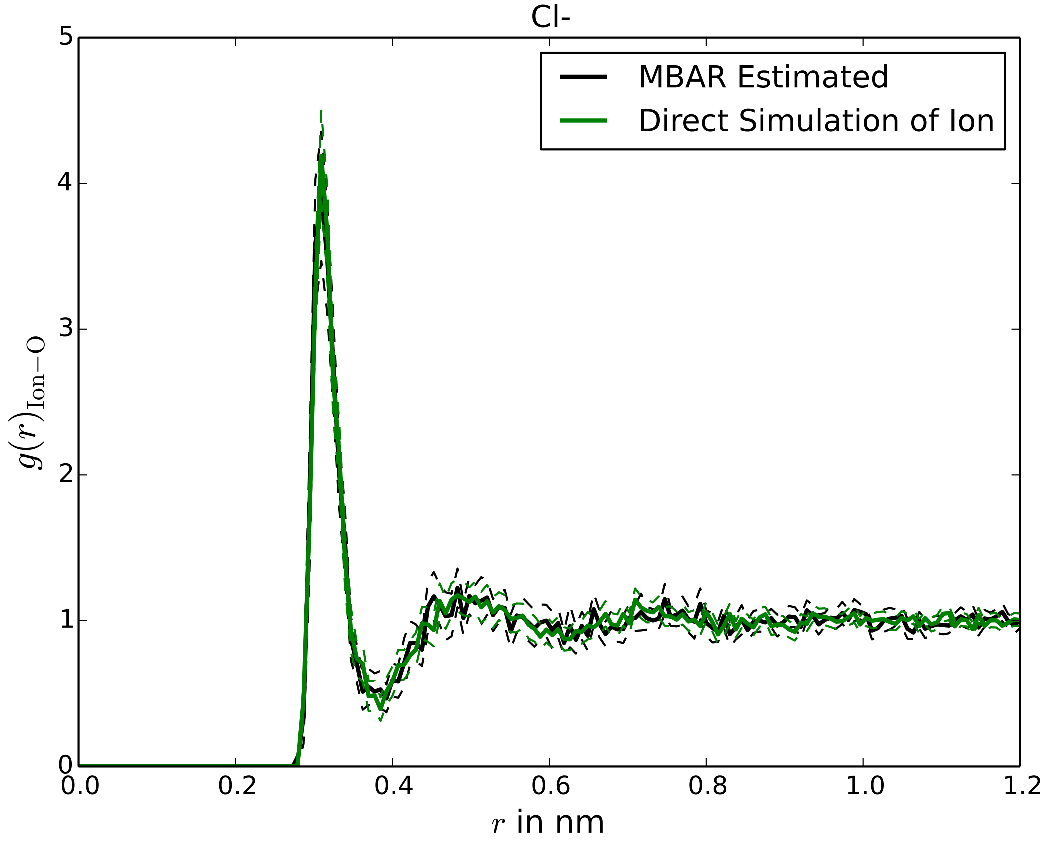


Figure S.7: RDF for $Cl^{-}$, this is also Fig. 8a

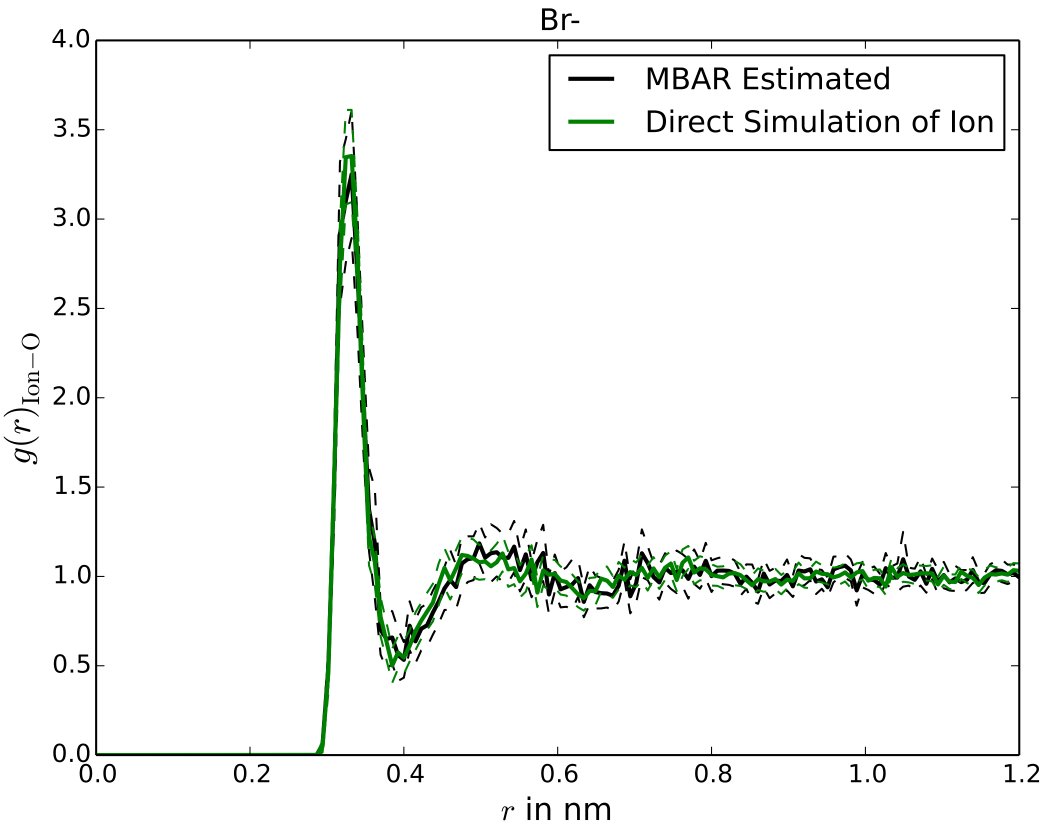


Figure S.8: RDF for $Br^-$

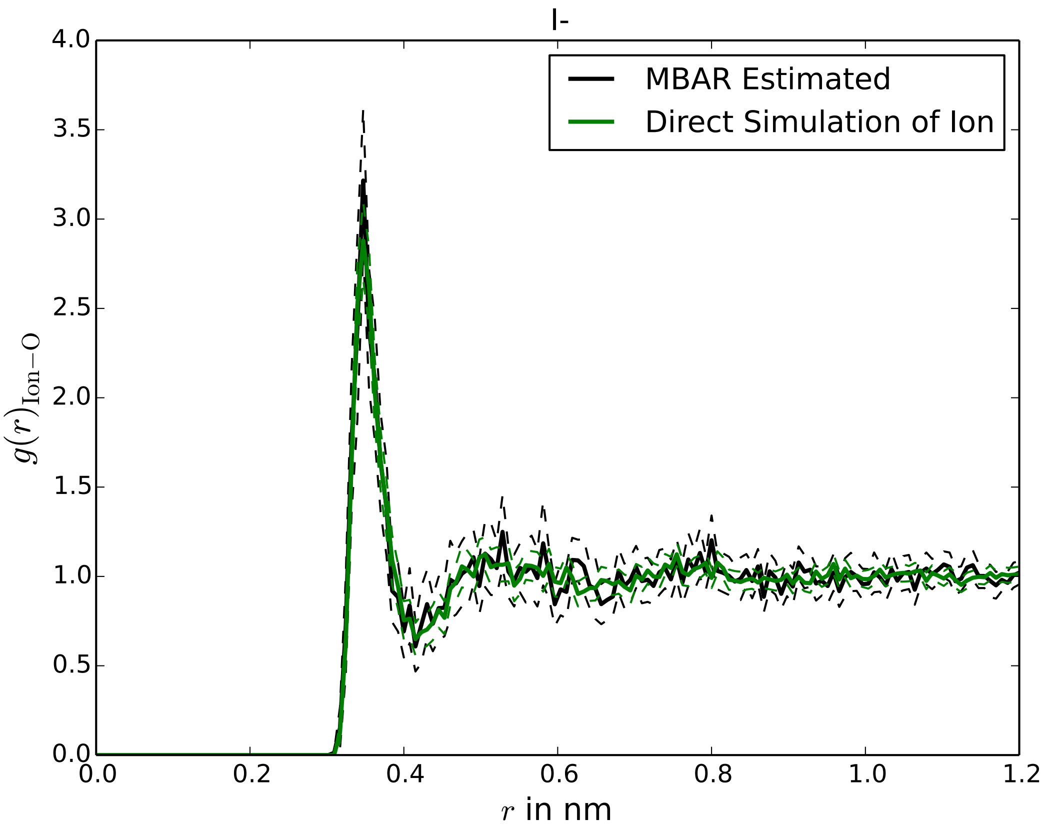


Figure S.9: RDF for $I^-$

## S.5 Sampled nonbonded parameter combination, mean and maximum uncertainty, and eigenvalues per iteration

Table S.2: All sampled parameters combinations, algorithm iteration from Section S.3, and eigenvalues ($\lambda$). Also shown is the maximum and mean uncertainty in the free energy per iteration. Algorithm attempts to create global phase space overlap to the reference state and samples regions of large uncertainty adaptively. New regions of low phase space overlap appear as jumps in the mean and maximum uncertainty and as eigenvalues of 1 to machine precision. Eigenvalues of the overlap matrix have a maximum of 1 and there will always be at least a eigenvalue of 1. The eigenvalues are shown as $1-\lambda$ to show how close each value is to 1, instead of repeated nines in the decimals. As such, the closer $1-\lambda$ is to zero, the closer $\lambda$ is to 1, indicating a lack of phase space overlap in sampled states. Uncertainty in free energy is in units of kcal/mol, partial charge ($q_i$) in units of $e^-$, $\varepsilon_{ij}$ in units of kcal/mol, and $\sigma_{ij}$ in units of nm.

| **Iteration** | **Max. Uncertainty** | **Mean Uncertainty** | **State Number** | $q_i$ | $\varepsilon_{ij}$ | $\sigma_{ij}$ | Minimum five $1-\lambda$ eigenvalues | | | | |
|---|---|---|---|---|---|---|---|---|---|---|---|
| Initial | 53.405 | 16.162 | 1 | 0.0000 | 0.0239 | 0.2500 | 0 | 0 | $7.00\cdot10^{-08}$ | $2.04\cdot10^{-03}$ | $1.22\cdot10^{-02}$ |
| | | | 2 | 0.0000 | 0.0501 | 0.5731 | | | | | |
| | | | 3 | 0.0000 | 0.0764 | 0.7120 | | | | | |
| | | | 4 | 0.0000 | 0.1027 | 0.8111 | | | | | |
| | | | 5 | 0.0000 | 0.1290 | 0.8906 | | | | | |
| | | | 6 | 0.0000 | 0.1553 | 0.9579 | | | | | |
| | | | 7 | 0.0000 | 0.1912 | 0.3000 | | | | | |
| | | | 8 | -2.0000 | 0.0501 | 0.5731 | | | | | |
| | | | 9 | -1.8516 | 0.0501 | 0.5731 | | | | | |
| | | | 10 | -1.6903 | 0.0501 | 0.5731 | | | | | |
| | | | 11 | -1.5119 | 0.0501 | 0.5731 | | | | | |
| | | | 12 | -1.3093 | 0.0501 | 0.5731 | | | | | |
| | | | 13 | -1.0690 | 0.0501 | 0.5731 | | | | | |
| | | | 14 | -0.7559 | 0.0501 | 0.5731 | | | | | |
| | | | 15 | 2.0000 | 0.0501 | 0.5731 | | | | | |
| | | | 16 | 1.8516 | 0.0501 | 0.5731 | | | | | |
| | | | 17 | 1.6903 | 0.0501 | 0.5731 | | | | | |
| | | | 18 | 1.5119 | 0.0501 | 0.5731 | | | | | |
| | | | 19 | 1.3093 | 0.0501 | 0.5731 | | | | | |
| | | | 20 | 1.0690 | 0.0501 | 0.5731 | | | | | |
| | | | 21 | 0.7559 | 0.0501 | 0.5731 | | | | | |

Continued on next page

Table S.2: Continued

| **Iteration** | **Max. Uncertainty** | **Mean Uncertainty** | **State Number** | $q_i$ | $\varepsilon_{ij}$ | $\sigma_{ij}$ | Minimum five $1-\lambda$ eigenvalues | | | | |
|---|---|---|---|---|---|---|---|---|---|---|---|
| 1 | 52.786 | 7.764 | 22 | -1.6798 | 0.6820 | 0.4889 | 0 | $1.90{\cdot}10^{-07}$ | $9.88{\cdot}10^{-05}$ | $5.07{\cdot}10^{-04}$ | $1.06{\cdot}10^{-03}$ |
| | | | 23 | -1.4749 | 0.4091 | 0.8854 | | | | | |
| | | | 24 | -0.8544 | 0.0790 | 0.7594 | | | | | |
| | | | 25 | 1.6595 | 0.5888 | 0.6613 | | | | | |
| | | | 26 | -0.5981 | 0.0704 | 0.7134 | | | | | |
| | | | 27 | 0.4314 | 0.1902 | 0.5986 | | | | | |
| | | | 28 | -1.6634 | 0.6602 | 0.5463 | | | | | |
| | | | 29 | -0.8917 | 0.0988 | 0.7682 | | | | | |
| 2 | 1.141 | 0.615 | 30 | -0.7029 | 0.6529 | 0.8259 | 0 | $1.18{\cdot}10^{-04}$ | $3.30{\cdot}10^{-04}$ | $6.78{\cdot}10^{-04}$ | $1.10{\cdot}10^{-03}$ |
| | | | 31 | 1.1703 | 0.8006 | 0.6868 | | | | | |
| | | | 32 | -0.0984 | 0.1345 | 0.6221 | | | | | |
| | | | 33 | 1.0954 | 0.7947 | 0.6935 | | | | | |
| 3 | 1.175 | 0.550 | 34 | -0.6410 | 0.4941 | 0.4167 | 0 | $1.80{\cdot}10^{-04}$ | $5.52{\cdot}10^{-04}$ | $9.29{\cdot}10^{-04}$ | $1.21{\cdot}10^{-03}$ |
| | | | 35 | 1.2092 | 0.1541 | 0.9427 | | | | | |
| | | | 36 | -0.3846 | 0.3165 | 0.4915 | | | | | |
| | | | 37 | 0.9190 | 0.1291 | 0.8801 | | | | | |
| 4 | 0.959 | 0.439 | 38 | -1.5202 | 0.1299 | 0.6784 | 0 | $3.45{\cdot}10^{-04}$ | $8.54{\cdot}10^{-04}$ | $1.18{\cdot}10^{-03}$ | $1.85{\cdot}10^{-03}$ |
| | | | 39 | 1.3982 | 0.1985 | 0.7431 | | | | | |
| | | | 40 | -1.3074 | 0.1187 | 0.6656 | | | | | |
| | | | 41 | 0.9507 | 0.1511 | 0.6975 | | | | | |
| 5 | 0.785 | 0.386 | 42 | -1.3734 | 0.5789 | 0.7564 | 0 | $3.22{\cdot}10^{-04}$ | $8.33{\cdot}10^{-04}$ | $1.33{\cdot}10^{-03}$ | $1.70{\cdot}10^{-03}$ |
| | | | 43 | 1.7199 | 0.4999 | 0.9266 | | | | | |
| | | | 44 | -1.2360 | 0.5260 | 0.7419 | | | | | |
| | | | 45 | -1.3115 | 0.5773 | 0.7606 | | | | | |

Continued on next page

Table S.2: Continued

| **Iteration** | **Max. Uncertainty** | **Mean Uncertainty** | **State Number** | $q_i$ | $\varepsilon_{ij}$ | $\sigma_{ij}$ | Minimum five $1-\lambda$ eigenvalues | | | | |
|---|---|---|---|---|---|---|---|---|---|---|---|
| 6 | 0.742 | 0.353 | 46 | -0.9298 | 0.5189 | 0.3859 | 0 | $3.45 \cdot 10^{-04}$ | $8.82 \cdot 10^{-04}$ | $1.59 \cdot 10^{-03}$ | $1.66 \cdot 10^{-03}$ |
| | | | 47 | -1.8873 | 0.0676 | 0.6959 | | | | | |
| | | | 48 | 1.9708 | 0.6180 | 0.7441 | | | | | |
| | | | 49 | -0.9112 | 0.5095 | 0.3917 | | | | | |
| | | | 50 | -0.2264 | 0.0522 | 0.5907 | | | | | |
| | | | 51 | -0.8718 | 0.5209 | 0.4012 | | | | | |
| 7 | 0.743 | 0.293 | 52 | -1.8748 | 0.4493 | 0.7703 | 0 | 0 | $4.56 \cdot 10^{-04}$ | $9.31 \cdot 10^{-04}$ | $1.54 \cdot 10^{-03}$ |
| | | | 53 | -1.4899 | 0.8230 | 0.3421 | | | | | |
| | | | 54 | 0.7295 | 0.6144 | 0.8865 | | | | | |
| | | | 55 | 1.5584 | 0.1116 | 0.8817 | | | | | |
| | | | 56 | 0.1870 | 0.0575 | 0.6282 | | | | | |
| | | | 57 | -1.5284 | 0.7857 | 0.4340 | | | | | |
| | | | 58 | -1.6665 | 0.4625 | 0.7809 | | | | | |
| | | | 59 | 1.5418 | 0.1217 | 0.8818 | | | | | |
| 8 | 0.698 | 0.287 | 60 | 0.3923 | 0.7698 | 0.3943 | 0 | 0 | $4.59 \cdot 10^{-04}$ | $9.64 \cdot 10^{-04}$ | $1.31 \cdot 10^{-03}$ |
| | | | 61 | 1.7228 | 0.1464 | 0.4531 | | | | | |
| | | | 62 | 1.6539 | 0.1425 | 0.4592 | | | | | |
| | | | 63 | 0.4455 | 0.7449 | 0.3970 | | | | | |
| 9 | 1.793 | 0.315 | 64 | 1.1971 | 0.1407 | 0.3559 | 0 | 0 | $1.04 \cdot 10^{-04}$ | $4.62 \cdot 10^{-04}$ | $9.65 \cdot 10^{-04}$ |
| | | | 65 | 1.0055 | 0.1262 | 0.4082 | | | | | |
| 10 | 0.839 | 0.285 | 66 | 1.4059 | 0.0609 | 0.2523 | 0 | 0 | 0 | $4.47 \cdot 10^{-04}$ | $9.51 \cdot 10^{-04}$ |
| | | | 67 | 0.7310 | 0.0557 | 0.4622 | | | | | |
| 11 | 0.816 | 0.284 | 68 | 1.9054 | 0.2172 | 0.2961 | 0 | 0 | 0 | 0 | $4.47 \cdot 10^{-04}$ |
| | | | 69 | 1.8673 | 0.2139 | 0.3079 | | | | | |

Continued on next page

Table S.2: Continued

| **Iteration** | **Max. Uncertainty** | **Mean Uncertainty** | **State Number** | $q_i$ | $\varepsilon_{ij}$ | $\sigma_{ij}$ | Minimum five $1-\lambda$ eigenvalues | | | | |
|---|---|---|---|---|---|---|---|---|---|---|---|
| 12 | 15.988 | 0.343 | 70 | -1.8691 | 0.1965 | 0.4437 | 0 | 0 | $1.38{\cdot}10^{-06}$ | $2.18{\cdot}10^{-04}$ | $6.19{\cdot}10^{-04}$ |
| | | | 71 | 1.3075 | 0.3699 | 0.2895 | | | | | |
| | | | 72 | -0.5981 | 0.0970 | 0.5383 | | | | | |
| | | | 73 | 1.1244 | 0.3251 | 0.3615 | | | | | |
| 13 | 15.988 | 0.332 | 74 | -1.9953 | 0.6150 | 0.4158 | 0 | 0 | $1.38{\cdot}10^{-06}$ | $4.99{\cdot}10^{-04}$ | $8.38{\cdot}10^{-04}$ |
| | | | 75 | -1.8357 | 0.5698 | 0.4330 | | | | | |
| 14 | 15.987 | 0.320 | 76 | -1.4563 | 0.1414 | 0.4190 | 0 | 0 | $1.38{\cdot}10^{-06}$ | $5.30{\cdot}10^{-03}$ | $9.56{\cdot}10^{-04}$ |
| | | | 77 | 1.6046 | 0.6396 | 0.3768 | | | | | |
| | | | 78 | -1.2524 | 0.1286 | 0.4475 | | | | | |
| | | | 79 | 1.2836 | 0.5217 | 0.4317 | | | | | |
| 15 | 1.549 | 0.292 | 80 | -1.8182 | 0.6459 | 0.3714 | 0 | 0 | $2.79{\cdot}10^{-04}$ | $4.74{\cdot}10^{-04}$ | $8.07{\cdot}10^{-04}$ |
| | | | 81 | -1.0881 | 0.3692 | 0.2903 | | | | | |
| | | | 82 | 1.4854 | 0.2016 | 0.3396 | | | | | |
| | | | 83 | 1.9247 | 0.4277 | 0.3114 | | | | | |
| | | | 84 | -1.0010 | 0.3436 | 0.3349 | | | | | |
| | | | 85 | 1.3963 | 0.1925 | 0.3637 | | | | | |
| | | | 86 | -1.7744 | 0.6293 | 0.3675 | | | | | |
| | | | 87 | 1.7226 | 0.3237 | 0.3250 | | | | | |
| 16 | 375.767 | 2.032 | 88 | -1.8046 | 0.2576 | 0.3012 | 0 | 0 | 0 | $5.90{\cdot}10^{-05}$ | $2.80{\cdot}10^{-04}$ |
| | | | 89 | -1.6602 | 0.2410 | 0.3426 | | | | | |
| 17 | 1.534 | 0.277 | 90 | -1.3695 | 0.1634 | 0.2763 | 0 | 0 | $7.98{\cdot}10^{-05}$ | $4.21{\cdot}10^{-04}$ | $8.07{\cdot}10^{-04}$ |
| | | | 91 | -1.2204 | 0.5042 | 0.3138 | | | | | |
| | | | 92 | -1.3421 | 0.1612 | 0.2902 | | | | | |
| | | | 93 | -1.3546 | 0.1975 | 0.2805 | | | | | |
| 18 | 1.499 | 0.277 | 94 | -1.7942 | 0.8037 | 0.2658 | 0 | 0 | $6.04{\cdot}10^{-05}$ | $4.21{\cdot}10^{-04}$ | $8.07{\cdot}10^{-04}$ |
| | | | 95 | -1.7583 | 0.7886 | 0.2809 | | | | | |

Continued on next page

## Table S.2: Continued

| Iteration | Max. Uncertainty | Mean Uncertainty | State Number | $q_i$ | $\varepsilon_{ij}$ | $\sigma_{ij}$ | Minimum five $1-\lambda$ eigenvalues | | | | |
|---|---|---|---|---|---|---|---|---|---|---|---|
| 19 | 0.925 | 0.273 | 96 | -1.3573 | 0.7020 | 0.2538 | 0 | 0 | $2.25{\cdot}10^{-04}$ | $5.76{\cdot}10^{-04}$ | $8.07{\cdot}10^{-04}$ |
| | | | 97 | -1.3301 | 0.6890 | 0.2705 | | | | | |
| 20 | 0.782 | 0.271 | 98 | -1.6690 | 0.6204 | 0.2839 | 0 | 0 | $2.53{\cdot}10^{-04}$ | $6.36{\cdot}10^{-04}$ | $8.08{\cdot}10^{-04}$ |
| | | | 99 | -1.5355 | 0.5748 | 0.3306 | | | | | |
| 21 | 0.716 | 0.251 | 100 | -1.9047 | 0.0793 | 0.3256 | 0 | 0 | $2.75{\cdot}10^{-04}$ | $7.74{\cdot}10^{-04}$ | $8.12{\cdot}10^{-04}$ |
| | | | 101 | -0.8341 | 0.7216 | 0.9577 | | | | | |
| | | | 102 | -1.7905 | 0.0775 | 0.3523 | | | | | |
| | | | 103 | -0.3003 | 0.2919 | 0.7587 | | | | | |
| 22 | 1.254 | 0.250 | 104 | -1.9806 | 0.1162 | 0.2766 | 0 | 0 | $2.35{\cdot}10^{-04}$ | $5.36{\cdot}10^{-04}$ | $7.33{\cdot}10^{-04}$ |
| | | | 105 | -1.9768 | 0.7723 | 0.5198 | | | | | |
| | | | 106 | -0.7425 | 0.5554 | 0.2759 | | | | | |
| | | | 107 | 0.8850 | 0.4370 | 0.2808 | | | | | |
| | | | 108 | -1.9014 | 0.1136 | 0.3031 | | | | | |
| | | | 109 | 0.8673 | 0.4293 | 0.2942 | | | | | |
| | | | 110 | -1.9028 | 0.7593 | 0.5108 | | | | | |
| | | | 111 | 0.7548 | 0.4465 | 0.2804 | | | | | |
| 23 | 0.811 | 0.249 | 112 | -1.7238 | 0.2068 | 0.2500 | 0 | 0 | $2.33{\cdot}10^{-04}$ | $6.59{\cdot}10^{-04}$ | $7.78{\cdot}10^{-04}$ |
| | | | 113 | -0.8728 | 0.3653 | 0.2734 | | | | | |
| | | | 114 | -0.7332 | 0.3148 | 0.3616 | | | | | |
| | | | 115 | -1.5707 | 0.2353 | 0.2545 | | | | | |
| 24 | 45.245 | 0.308 | 116 | -1.8840 | 0.5348 | 0.2500 | 0 | $3.40{\cdot}10^{-07}$ | $2.29{\cdot}10^{-04}$ | $6.65{\cdot}10^{-04}$ | $7.94{\cdot}10^{-04}$ |
| | | | 117 | -2.0000 | 0.7852 | 0.8961 | | | | | |
| | | | 118 | 1.8905 | 0.3243 | 0.2500 | | | | | |
| | | | 119 | -1.7333 | 0.4960 | 0.3088 | | | | | |
| | | | 120 | 1.8149 | 0.3133 | 0.2824 | | | | | |
| | | | 121 | -1.8864 | 0.5398 | 0.3097 | | | | | |

Continued on next page

## Table S.2: Continued

| Iteration | Max. Uncertainty | Mean Uncertainty | State Number | $q_i$ | $\varepsilon_{ij}$ | $\sigma_{ij}$ | Minimum five $1-\lambda$ eigenvalues | | | | |
|---|---|---|---|---|---|---|---|---|---|---|---|
| 25 | 0.712 | 0.235 | 122 | -1.8495 | 0.0742 | 0.7687 | 0 | $2.20\cdot10^{-04}$ | $5.66\cdot10^{-04}$ | $7.48\cdot10^{-04}$ | $2.12\cdot10^{-03}$ |
| | | | 123 | 1.2859 | 0.1263 | 0.2500 | | | | | |
| | | | 124 | 1.1208 | 0.8537 | 0.9557 | | | | | |
| | | | 125 | 1.9858 | 0.7161 | 0.2500 | | | | | |
| | | | 126 | -0.9987 | 0.7161 | 0.2500 | | | | | |
| | | | 127 | 1.2345 | 0.1233 | 0.2824 | | | | | |
| | | | 128 | 1.5659 | 0.3622 | 0.2500 | | | | | |
| | | | 129 | 1.9858 | 0.7161 | 0.2500 | | | | | |
| 26 | 4.200 | 0.237 | 130 | -1.7965 | 0.0761 | 0.2500 | 0 | $1.76\cdot10^{-05}$ | $1.98\cdot10^{-04}$ | $5.19\cdot10^{-04}$ | $6.48\cdot10^{-04}$ |
| | | | 131 | -1.1030 | 0.1372 | 0.2500 | | | | | |
| | | | 132 | -0.5576 | 0.0754 | 0.2500 | | | | | |
| | | | 133 | 0.6581 | 0.2799 | 0.2500 | | | | | |
| | | | 134 | -0.5464 | 0.2799 | 0.2672 | | | | | |
| | | | 135 | 0.6318 | 0.2707 | 0.2824 | | | | | |
| | | | 136 | -1.7410 | 0.0810 | 0.2500 | | | | | |
| | | | 137 | -1.0048 | 0.1261 | 0.2500 | | | | | |
| 27 | 1.024 | 0.233 | 138 | -1.5042 | 0.0268 | 0.2500 | 0 | $1.68\cdot10^{-04}$ | $3.27\cdot10^{-04}$ | $5.22\cdot10^{-04}$ | $6.89\cdot10^{-04}$ |
| | | | 139 | -1.1001 | 0.0268 | 0.2500 | | | | | |
| | | | 140 | 2.0000 | 0.8516 | 0.8046 | | | | | |
| | | | 141 | -1.0341 | 0.2125 | 0.2962 | | | | | |
| | | | 142 | 1.8800 | 0.8035 | 0.7942 | | | | | |
| | | | 143 | -1.3829 | 0.0856 | 0.2500 | | | | | |

Continued on next page

# Table S.2: Continued

| **Iteration** | **Max. Uncertainty** | **Mean Uncertainty** | **State Number** | $q_i$ | $\varepsilon_{ij}$ | $\sigma_{ij}$ | Minimum five $1-\lambda$ eigenvalues | | | | |
|---|---|---|---|---|---|---|---|---|---|---|---|
| 28 | 0.716 | 0.233 | 144 | -1.7489 | 0.0677 | 0.2500 | 0 | $1.65{\cdot}10^{-04}$ | $4.96{\cdot}10^{-04}$ | $6.38{\cdot}10^{-04}$ | $1.40{\cdot}10^{-03}$ |
| | | | 145 | -1.9845 | 0.2315 | 0.3688 | | | | | |
| | | | 146 | -1.2066 | 0.0742 | 0.2500 | | | | | |
| | | | 147 | -1.1825 | 0.0737 | 0.2672 | | | | | |
| | | | 148 | -1.8101 | 0.1103 | 0.2909 | | | | | |
| | | | 149 | -1.5320 | 0.0703 | 0.2500 | | | | | |
| 29 | 0.641 | 0.233 | 150 | -1.9604 | 0.2006 | 0.2500 | 0 | $1.49{\cdot}10^{-04}$ | $4.66{\cdot}10^{-04}$ | $6.41{\cdot}10^{-04}$ | $1.66{\cdot}10^{-03}$ |
| | | | 151 | -1.1793 | 0.0288 | 0.2500 | | | | | |
| | | | 152 | -0.7656 | 0.0534 | 0.2500 | | | | | |
| | | | 153 | 0.8766 | 0.0515 | 0.2500 | | | | | |
| | | | 154 | 1.6513 | 0.0648 | 0.2728 | | | | | |
| | | | 155 | -0.7503 | 0.0533 | 0.2672 | | | | | |
| | | | 156 | 0.8064 | 0.0514 | 0.3088 | | | | | |
| | | | 157 | -1.3043 | 0.0563 | 0.2500 | | | | | |
| | | | 158 | -1.0469 | 0.0367 | 0.2500 | | | | | |
| | | | 159 | 0.9076 | 0.0520 | 0.2510 | | | | | |
| 30 | 0.641 | 0.199 | 160 | 0.6764 | 0.8382 | 0.3336 | 0 | $1.60{\cdot}10^{-04}$ | $5.41{\cdot}10^{-04}$ | $1.11{\cdot}10^{-03}$ | $1.71{\cdot}10^{-03}$ |
| | | | 161 | 1.4891 | 0.2481 | 0.9246 | | | | | |
| | | | 162 | 0.6629 | 0.8224 | 0.3424 | | | | | |
| | | | 163 | 0.4765 | 0.1135 | 0.7249 | | | | | |
| . 31 | 0.636 | 0.168 | 164 | 1.8978 | 0.2442 | 0.7260 | 0 | $1.79{\cdot}10^{-04}$ | $6.66{\cdot}10^{-04}$ | $1.49{\cdot}10^{-03}$ | $1.85{\cdot}10^{-03}$ |
| | | | 165 | -1.6132 | 0.6120 | 0.5550 | | | | | |
| | | | 166 | -1.2083 | 0.3974 | 0.8977 | | | | | |
| | | | 167 | 0.6832 | 0.1200 | 0.6369 | | | | | |
| | | | 168 | -1.0002 | 0.3985 | 0.5621 | | | | | |
| | | | 169 | -1.4755 | 0.5390 | 0.5621 | | | | | |

Continued on next page

Table S.2: Continued

| **Iteration** | **Max. Uncertainty** | **Mean Uncertainty** | **State Number** | $q_i$ | $\varepsilon_{ij}$ | $\sigma_{ij}$ | Minimum five $1-\lambda$ eigenvalues | | | | |
|---|---|---|---|---|---|---|---|---|---|---|---|
| 32 . | 0.638 | 0.162 | 170 | 1.6020 | 0.2264 | 0.4529 | 0 | $7.73 \cdot 10^{-04}$ | $1.51 \cdot 10^{-03}$ | $1.85 \cdot 10^{-03}$ | $1.87 \cdot 10^{-03}$ |
| | | | 171 | 0.2884 | 0.0819 | 0.5552 | | | | | |
| 33 | 0.636 | 0.158 | 172 | -1.3653 | 0.4527 | 0.9329 | 0 | $1.84 \cdot 10^{-04}$ | $7.97 \cdot 10^{-04}$ | $1.57 \cdot 10^{-03}$ | $1.93 \cdot 10^{-03}$ |
| | | | 173 | 1.7108 | 0.3400 | 0.3091 | | | | | |
| | | | 174 | -0.2731 | 0.1307 | 0.6790 | | | | | |
| | | | 175 | 1.5397 | 0.3110 | 0.6790 | | | | | |
| 34 | 0.634 | 0.151 | 176 | -1.7402 | 0.1735 | 0.2968 | 0 | $1.83 \cdot 10^{-04}$ | $8.48 \cdot 10^{-04}$ | $1.61 \cdot 10^{-03}$ | $1.93 \cdot 10^{-03}$ |
| | | | 177 | 0.7764 | 0.8525 | 0.9370 | | | | | |
| | | | 178 | 1.5458 | 0.1252 | 0.6505 | | | | | |
| | | | 179 | -1.1485 | 0.1316 | 0.4332 | | | | | |
| | | | 180 | 1.0821 | 0.1028 | 0.6292 | | | | | |
| | | | 181 | 1.5304 | 0.1398 | 0.6590 | | | | | |
| 35 | 0.634 | 0.141 | 182 | -0.8934 | 0.6479 | 0.8374 | 0 | $1.82 \cdot 10^{-04}$ | $8.81 \cdot 10^{-04}$ | $1.64 \cdot 10^{-03}$ | $2.02 \cdot 10^{-03}$ |
| | | | 183 | 1.6751 | 0.1045 | 0.3914 | | | | | |
| | | | 184 | -0.5360 | 0.4088 | 0.7534 | | | | | |
| | | | 185 | 1.2396 | 0.0904 | 0.4536 | | | | | |
| 36 | 0.634 | 0.138 | 186 | -1.2996 | 0.6071 | 0.6355 | 0 | $1.82 \cdot 10^{-04}$ | $8.68 \cdot 10^{-04}$ | $1.63 \cdot 10^{-03}$ | $1.97 \cdot 10^{-03}$ |
| | | | 187 | 1.8999 | 0.7088 | 0.5807 | | | | | |
| | | | 188 | -1.1696 | 0.5514 | 0.6298 | | | | | |
| | | | 189 | 1.8360 | 0.7067 | 0.5819 | | | | | |
| 37 | 0.633 | 0.127 | 190 | -1.7443 | 0.2920 | 0.6633 | 0 | $1.85 \cdot 10^{-04}$ | $8.80 \cdot 10^{-04}$ | $1.67 \cdot 10^{-03}$ | $2.17 \cdot 10^{-03}$ |
| | | | 191 | 0.5927 | 0.5728 | 0.9083 | | | | | |
| | | | 192 | -0.1047 | 0.0647 | 0.5794 | | | | | |
| | | | 193 | 0.2188 | 0.5279 | 0.8777 | | | | | |

Continued on next page

Table S.2: Continued

| Iteration | Max. Uncertainty | Mean Uncertainty | State Number | $q_i$ | $\varepsilon_{ij}$ | $\sigma_{ij}$ | Minimum five $1-\lambda$ eigenvalues | | | | |
|---|---|---|---|---|---|---|---|---|---|---|---|
| 38 | 0.633 | 0.123 | 194 | -1.9705 | 0.7639 | 0.8696 | 0 | $1.84{\cdot}10^{-04}$ | $8.78{\cdot}10^{-04}$ | $1.66{\cdot}10^{-03}$ | $2.16{\cdot}10^{-03}$ |
| | | | 195 | 1.7253 | 0.5893 | 0.9258 | | | | | |
| | | | 196 | 0.0345 | 0.0610 | 0.5852 | | | | | |
| | | | 197 | -1.7487 | 0.7534 | 0.8732 | | | | | |
| 39 | 0.633 | 0.119 | 198 | -1.6028 | 0.7917 | 0.8307 | 0 | $1.84{\cdot}10^{-04}$ | $9.30{\cdot}10^{-04}$ | $1.68{\cdot}10^{-03}$ | $2.21{\cdot}10^{-03}$ |
| | | | 199 | 1.3667 | 0.4290 | 0.5441 | | | | | |
| | | | 200 | 0.1093 | 0.0805 | 0.5710 | | | | | |
| | | | 201 | 1.3073 | 0.4362 | 0.5533 | | | | | |
| 40 | 0.631 | 0.118 | 202 | -1.3977 | 0.3683 | 0.5108 | 0 | $1.89{\cdot}10^{-04}$ | $9.21{\cdot}10^{-04}$ | $1.70{\cdot}10^{-03}$ | $2.24{\cdot}10^{-03}$ |
| | | | 203 | -1.0064 | 0.2793 | 0.5297 | | | | | |

## S.6 Corrections to Simulation Free Energies for Comparison to Born Solvation Model

The choice of simulation parameters and settings introduces various errors which will change the free energy estimate in predictable ways. Many of the calculations performed in this study were between simulations carried out under the same boundary conditions, ensembles, electrostatic treatment, etc. Removing these errors introduced from the simulation settings would therefore apply to all results, and only shift the answer, but not the difference in properties, such as free energy differences. If we want to compare the free energy estimate between methods, we must correct the simulated results to provide a methodological independent free energy estimate. One example of these corrections is the ideal gas expansion comparison simulations and experimental results that we accounted for in the results from Joung and Cheatham in Section 4.4.2.

Comparing our free energy estimates from simulation to the Born approximation to solvation free energy requires removing the methodological dependence from our simulations. Hünenberger and Reif provide an excellent account of all the neglected physical factors in the Born model, and how to remove the methodological dependence for atomistic simulations.[18] This section details the corrections we applied to our free energy estimates. The result of the these corrections and the comparison of our simulation to the Born approximation are shown in Section 4.4.4. We use the similar terminology and variables as in Hünenberger and Reif, but not exact; as such, we show which equations and tables in the source material these corrections came from inside angle braces: e.g. {Eq. 6.1}. As a reminder, we ran with periodic boundary conditions under a lattice-sum electrostatics scheme.

The free energy of solvation, $\Delta F$ is

$$\Delta_s G = \Delta_s G_{chg}^{raw} + \Delta_s G_{cor} + \Delta_s G_{cav} + \Delta_s G_{std} \tag{S.6}$$

where the subscript $s$ stands for simulation, $\Delta_s G_{chg}^{raw}$ is the free energy estimate of charging an ion of

fixed size from zero charge, $\Delta_s G_{cor}$ are the correction terms to remove methodological dependence, and $\Delta_s G_{std}$ is the isothermal ideal-gas compression at standard state {Eq. 6.42}. Our comparison to the Born model was a deviation of the Born model to our results for charging only. This means that we subtracted off the free energy of the uncharged particle of the same size for both models, removing the need to calculate $\Delta_s G_{cav}$ and $\Delta_s G_{std}$ as they would cancel out of the calculation. $\Delta_s G_{cor}$ for periodic boundary conditions with lattice-sum electrostatics is

$$\Delta_s G_{cor} = \Delta_s G_B + \Delta_s G_{C1} + \Delta_s G_{C2} + \Delta_s G_D \tag{S.7}$$

where each term on the right hand side corresponds to a different type of correction {Eq. 6.43} which we detail below.

$\Delta_s G_B$ removes the error in solvent polarization introduced from the finite simulated system size and periodicity. This correction is analytical for the spherical ion surrounded by a periodic lattice-sum solvent and is {Eq. 6.20} of the source material as

$$\begin{aligned} \Delta_s G_B = {} & (8\pi\varepsilon_0)^{-1} N_A q^2 \left(1 - \varepsilon_d^{-1}\right) L^{-1} \\ & \times \left[\alpha_{LS} + \frac{4\pi}{3}\left(\frac{R_{ij}}{L}\right)^3 - \frac{16\pi^2}{45}\left(\frac{R_{ij}}{L}\right)^5\right] \end{aligned} \tag{S.8}$$

where $\varepsilon_0$ is the dielectric of vacuum, $N_A$ is Avogadro's constant, $q$ is the charge of the solute particle in units of elementary charge $e$, $\varepsilon_d = 92$ is the model solvent dielectric for TIP3P water,[19] $L$ is the average box length for the cubic simulation box evaluated at an uncharged particle of the same size, $\alpha_{LS} \approx -2.837297$ is the lattice-sum self-term constant {Eq. 3.28}, and $R_{ij}$ is the Born radius which we assume is the effective hard sphere (EHS) radius as we computed in Section 4.4.4.

$\Delta_s G_{C1}$ corrects for the error introduced by evaluating the electrostatics from of complete molecules up to a cutoff, instead of evaluating up to a spherical cutoff discarding atoms outside the cutoff, but bound to a fragment of the molecule inside the cutoff {Section 3.3.3}. We evaluate this correction

by substituting {Eq. 6.27 and Eq. 6.45} into {Eq. 6.30}

$$\Delta_s G_{C1} \approx \frac{-N_A q (N_S + 1)}{6\varepsilon_0 L^3} \left(1 - \frac{4\pi R_{ij}^3}{3L^3}\right) \mathscr{Q} \tag{S.9}$$

where $N_S$ is the number of solvent molecules, and $\mathscr{Q} = 7.64 \cdot 10^{-3} e \cdot nm^2$ is the quadrupole-moment trace of the TIP3P water model {Table 3.1}.

$\Delta_s G_{C2}$ corrects for the vanishing average potential in the lattice-sum model as the potential is evaluated towards the edge of the box. This results in an omitted zero term in the Fourier series and offsets the potential at the solute center. The lattice-sum correction is {Eq. 6.37} and

$$\Delta_s G_{C2} = -N_A q \frac{4\pi R_{ij}^3}{3L^3} \left(\chi_S + \frac{\tilde{\chi}_{S-}}{R_{ij}}\right) \tag{S.10}$$

where $\chi_S = 0.73V$ is the interface potential at a planar air-liquid interface measured in the air-to-liquid direction, and $\tilde{\chi}_{S-} = -0.11V \cdot nm$ is a factor characterizing the near approximate linear dependence of the air-liquid interface potential measured in the same direction. The values used for $\chi_S$ and $\tilde{\chi}_{S-}$ are taken from SPC water at 300K as these were the data available, so $\Delta_s G_{C2}$ is an approximation for our purposes.

$\Delta_s G_D$ corrects for the fact that the solvent model relative dielectric, $\varepsilon_d$, differs from the experimental relative dielectric, $\varepsilon_e$. In the case of water, $\varepsilon_e = 78.36$ {Table 1.1}. We compute this correction term as {Eq. 6.41} and

$$\Delta_s G_D = \frac{N_A q^2 \left(\varepsilon_e^{-1} - \varepsilon_d^{-1}\right)}{8\pi\varepsilon_0 R_{ij}} \tag{S.11}$$

Finally, combining all of these corrections into our simulated results allows us to make a methodologically independent comparison between our results and the Born approximation to solvation free energy.

## References

(1) Naden, L. N.; Pham, T. T.; Shirts, M. R. *J. Chem. Theory Comput.* **2014**, *10*, 1128–1149.

(2) Kaminski, G. A.; Friesner, R. A.; Tirado-rives, J.; Jorgensen, W. L. *J. Phys. Chem. B* **2001**, *2*, 6474–6487.

(3) Shirts, M. R.; Pande, V. S. *J. Chem. Phys.* **2005**, *122*, 144107.

(4) Paliwal, H.; Shirts, M. R. *J. Chem. Theory Comput.* **2011**, 4115–4134.

(5) Kuharski, R. A.; Rossky, P. J. *J. Am. Chem. Soc.* **1984**, *106*, 5794–5800.

(6) Beutler, T.; Mark, A.; van Schaik, R. *Chem. Phys. Lett.* **1994**, *222*, 529–539.

(7) Zacharias, M.; Straatsma, T. P.; McCammon, J. A. *J. Chem. Phys.* **1994**, *100*, 9025.

(8) Pham, T. T.; Shirts, M. R. *J. Chem. Phys.* **2011**, *135*, 034114.

(9) Pham, T. T.; Shirts, M. R. *J. Chem. Phys.* **2012**, *136*, 124120.

(10) Analysis code for this project can be found in the ion-parameter repository on GitHub at `https://github.com/shirtsgroup/ion-parameters` with commit hash 7ff188b0bc or later.

(11) Shirts, M. R.; Chodera, J. D. *J. Chem. Phys.* **2008**, *129*, 124105.

(12) Ester, M.; Kriegel, H.-p.; S, J.; Xu, X. A density-based algorithm for discovering clusters in large spatial databases with noise. 1996.

(13) SciPy: Open Source Scientific Tools for Python. `http://www.scipy.org/` (accessed May 3, 2014).

(14) Kruskal, J. B. *Proc. Am. Math. Soc.* **1956**, *7*, 48–50.

(15) Sobel, I.; Feldman, G. "A 3x3 Isotropic Gradient Operator for Image Processing. 1968.

(16) Joung, I. S.; Cheatham, T. E. *J. Phys. Chem. B* **2008**, *112*, 9020–41.

(17) Efron, B.; Tibshirani, R. *An Introduction to the Bootstrap*; Chapman & Hall/CRC, 1993; p 436.

(18) Hünenberger, P.; Reif, M. *Single-Ion Solvation: Experimental and Theoretical Approaches to Elusive Thermodynamic Quantities*; RSC theoretical and computational chemistry series; Royal Society of Chemistry, 2011.

(19) Lamoureux, G.; a.D. MacKerell,; Roux, B. *J. Chem. Phys.* **2003**, *119*, 5185–5197.
